# Supplementary material for: Approximate Inference Turns Deep Networks into Gaussian Processes
Source: arXiv:1906.01930 source file (2020-07-19)

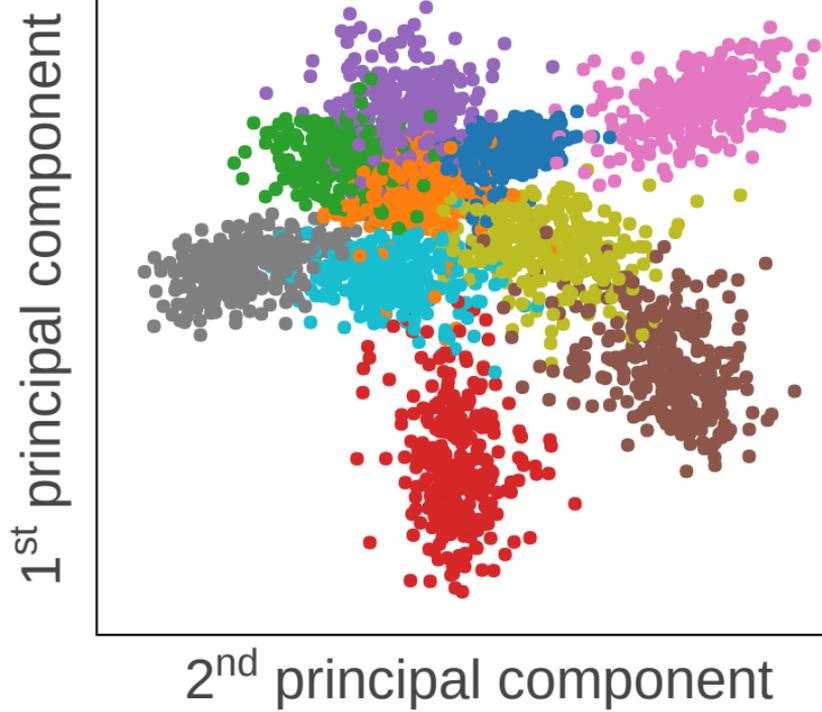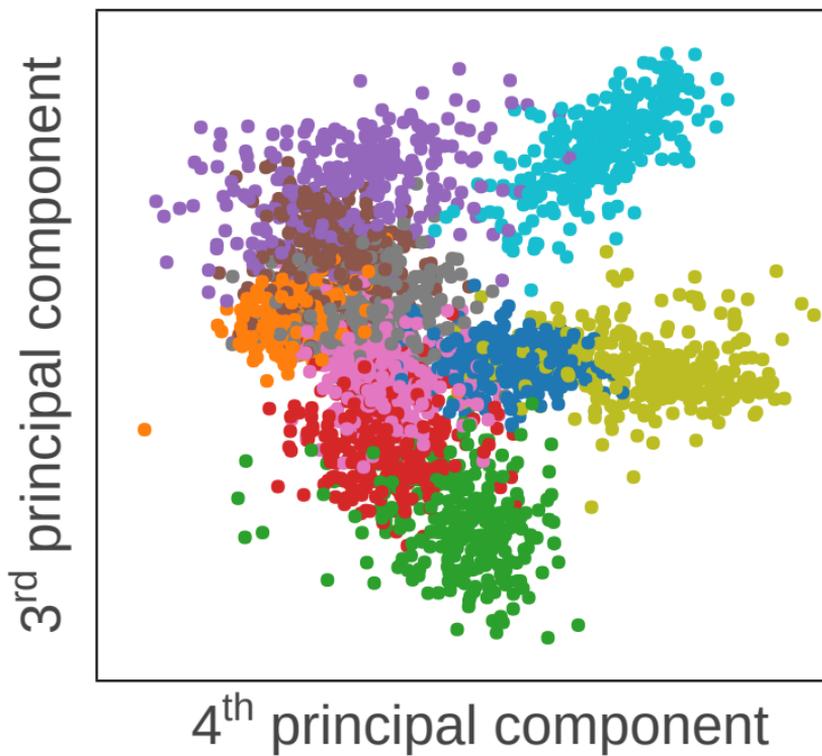

Supplement: Supplementary file 3 [file mnist_l2adalex_pca.pdf]
