# Supplementary material for: Approximate Inference Turns Deep Networks into Gaussian Processes
Source: arXiv:1906.01930 source file (2020-07-19)
Supplement: Supplementary file 4 [file mnist_vogn_pca.pdf]

1<sup>st</sup> principal component

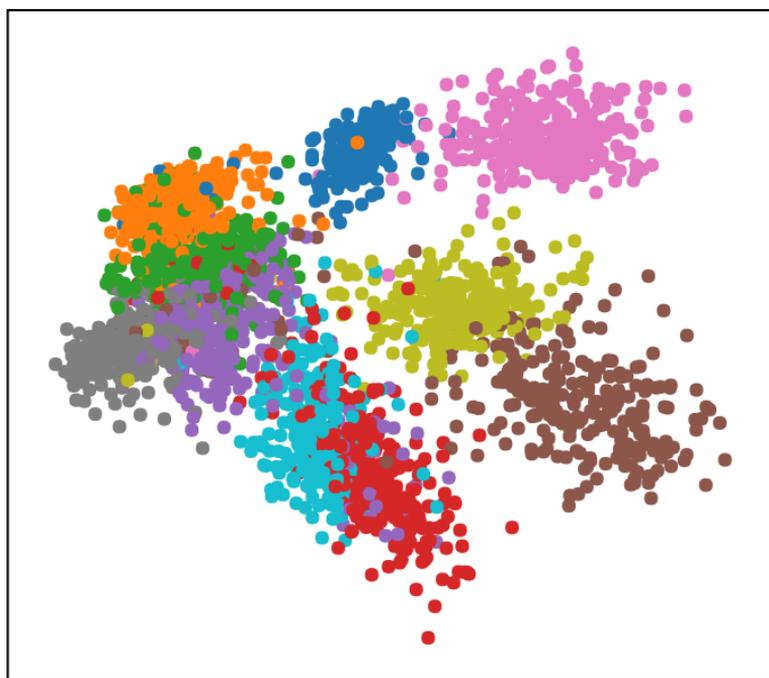

2<sup>nd</sup> principal component

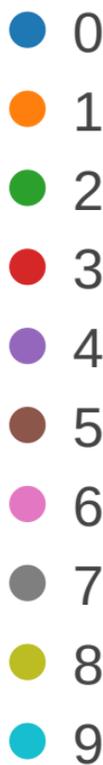

3<sup>rd</sup> principal component

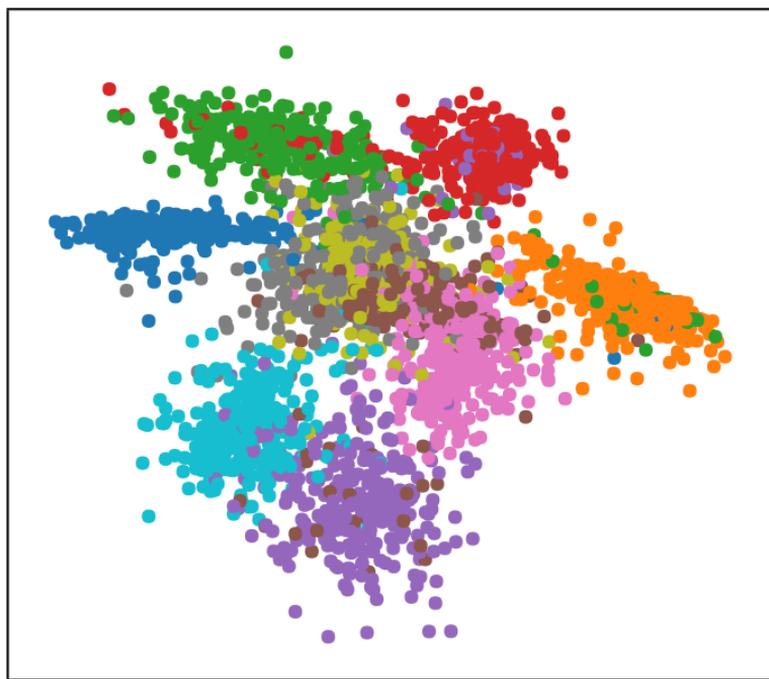

4<sup>th</sup> principal component
