# Supplementary material for: Approximate Inference Turns Deep Networks into Gaussian Processes
Source: arXiv:1906.01930 source file (2020-07-19)
Supplement: Supplementary file 5 [file _app_AA_old_proofs.tex]

\begin{restatable}{thm}{thmviiter}
    \label{thm:vi_iter}
    {\bf (Iterations of a VI algorithm as a GP) :} At each iteration $t$ of the VOGGN update, i.e. \eqref{eq:ngvi_update_1} and \eqref{eq:ngvi_update_2} but with the GGN approximation to the Hessian, the posterior approximation $q_t(\vparam) := \gauss(\vparam|\vmu_t,\vSigma_t)$ is equivalent to the posterior distribution of the following linear basis-function model:
        \begin{align}
            \tvy_{i,s} &= \vJ_s(\vx_i)\vparam + \vepsilon_{i,s}, \textrm{ with }  \vepsilon_{i,s} \sim \gauss(0, S(\beta_t\vLambda_{i,s})^{-1})
            \textrm{ and } \vparam \sim \gauss(\vm_t,\vS_t)
        \end{align}
    where $\vS_t^{-1} := (1-\beta_t)\vSigma_t^{-1} + \beta_t \delta \vI_P$ and $\vm_t := (1-\beta_t)\vS_t\vSigma_t^{-1}\vmu_t$.
    The observations are defined as $\tvy_{i,s} := \vJ_s(\vx_i)\vmu_t - \vLambda_{i,s}^{-1}\vr_{i,s}$ and the feature maps are defined as $\vJ_s(\vx_i)^\top$ with $\vJ_s(\vx_i)$, $\vr_{i,s}$, and $\vLambda_{i,s}$ denoting the Jacobian, residual, and noise precision evaluated at the sampled weight $\vparam^{(s)}$ drawn from $q_t(\vparam)$.
    The predictive distribution of this model is equivalent to that of the following GP regression model:
    \begin{align}
        \tvy_{i,s} = \vf_s(\vx_i) + \vepsilon_{i,s},
        \quad \textrm{ where } \vf_s(\vx) \sim \mathcal{GP}\rnd{ \vJ_s(\vx)\vm_t, \vJ_s(\vx) \vS_t \vJ_{s'}(\vx')^\top} .
    \end{align}
\end{restatable}



\subsection{Proof of Theorem \ref{thm:vi_ggn}}\label{proof:thmviggn}
\begin{restatable}{thm}{thmviggn}
    \label{thm:vi_ggn}
    {\bf (Minima of the variational objectives as a GP) :}
    The Variational-GGN-MC approximation $\Tilde{q}_*(\vparam)$ as defined above is equivalent to the posterior distribution of a linear basis-function model with observations $\tvy_{i,s} \in\real^K$:
        \begin{align}
            \tvy_{i,s} &= \vJ_s(\vx_i)\vparam + \vepsilon_{i,s}, \textrm{ with }  \vepsilon_{i,s} \sim \gauss(0, S\vLambda_{i,s}^{-1})
            \textrm{ and } \vparam \sim \gauss(0,\delta^{-1}\vI_P),
        \end{align}
    where the observations are defined as $\tvy_{i,s} := \vJ_s(\vx_i)\vmu_* - \vLambda_{i,s}^{-1}\vr_{i,s}$ and the feature maps are defined as $\vJ_s(\vx_i)^\top$ with $\vJ_s(\vx_i)$, $\vr_{i,s}$, and $\vLambda_{i,s}$ denoting the Jacobian, residual, and noise precision evaluated at the sampled weight $\vparam^{(s)}$ drawn from $\Tilde{q}_*(\vparam)$.
    The predictive distribution of this model is equivalent to that of the following GP regression model:
    \begin{align}
        \tvy_{i,s} = \vf_s(\vx_i) + \vepsilon_{i,s},
        \quad \textrm{ where } \vf_s(\vx) \sim \mathcal{GP}\rnd{ 0, \delta^{-1} \vJ_s(\vx) \vJ_{s'}(\vx')^\top}. 
    \end{align}
\end{restatable} 

\begin{proof}
We prove this theorem in the same way as we did for the previous one. Let $\veta_* := \{ \vSigma_*^{-1} \vmu_*, -\half\vSigma_*^{-1} \}$ denote the natural-parameters of the Variational approximation $q_*(\vparam) := \gauss(\vparam|\vmu_*,\vSigma_*)$ that satisfies the condition \eqref{eq:vi_stationary}. We first find $\veta_*$ and then obtain the distribution. For the expectations in \eqref{eq:vi_stationary}, we use Monte Carlo sampling. The second natural parameter then is
\begin{align}
    -\half \vSigma_*^{-1}
    & = -\half \sqr{\sum_{i=1}^N \myexpect_{q_*(\param)} \sqr{ \nabla_{\param\param}^2 \loss_i(\vparam)} + \delta \vI_P}
    & \approx  -\half \sqr{ \frac{1}{S} \sum_{i,s = 1}^{N,S} \nabla_{\param\param}^2 \loss_i(\vparam^{(s)}) + \delta \vI_P }.
    \label{eq:nat_param_2_vi}
\end{align}
Using the first condition of \eqref{eq:vi_stationary}, the first natural parameter can be written as
\begin{align}
    \vSigma_*^{-1}\vmu_* &= -\sum_{i=1}^N \myexpect_{q_*(\param)} \sqr{ \nabla_\param \loss_i(\vparam) } - \delta \vmu_*  + \vSigma_*^{-1}\vmu_* \\
    &\approx - \frac{1}{S} \sum_{i,s = 1}^{N,S} \nabla_\param \loss_i(\vparam^{(s)}) -\delta \vmu_*  + \sqr{ \frac{1}{S} \sum_{i,s = 1}^{N,S} \nabla_{\param\param}^2 \loss_i(\vparam^{(s)}) + \delta \vI_P }\vmu_* \\
    &= \frac{1}{S} \sum_{i,s = 1}^{N,S} \sqr{ -\nabla_\param \loss_i(\vparam^{(s)}) + \nabla_{\param\param}^2 \loss_i(\vparam^{(s)})  \vmu_* } .
    \label{eq:nat_param_1_vi}
\end{align}
The equations above are similar to the natural parameters of the Laplace approximation \eqref{eq:nat_param_2_laplace} and \eqref{eq:nat_param_1_laplace} except that we have another sum which is taken over the samples $(s)$. We can treat them as observations. Given \eqref{eq:nat_param_2_vi} and \eqref{eq:nat_param_1_vi}, the Variational-MC approximation $q_*(\vparam)$ is thus proportional to 
\begin{align}
   % q_* &\propto \exp{ \sqr{  - \half \vparam^\top \vSigma_*^{-1}\vparam + \vparam^\top\vSigma_*^{-1}\vmu_* } } \\
   \exp{\rnd{ \frac{-\delta \vparam^\top\vparam}{2} }} \prod_{i,s = 1}^{N,S} \exp{ \sqr{ - \frac{1}{2S} \vparam^\top \nabla_{\param\param}^2 \loss_i(\vparam^{(s)})\vparam + \frac{\vparam^\top}{S}  \crl{ -\nabla_\param \loss_i(\vparam^{(s)}) + \nabla_{\param\param}^2 \loss_i(\vparam^{(s)})  \vmu_* }  } }.
\end{align}
Here again, the key step is that we can use the GGN approximation \eqref{eq:ggn} to show that the Variational-GGN-MC approximation $\Tilde{q}_*(\vparam)$ is proportional to
\be
\exp{\rnd{ \frac{-\delta \vparam^\top\vparam}{2} }} \prod_{i,s = 1}^{N,S} \exp{ \sqr{ - \half \vparam^\top \vJ_s(\vx_i)^\top \frac{\vLambda_{i,s}}{S} \vJ_s(\vx_i) \vparam +\frac{\vparam^\top \vJ_s(\vx_i)^\top}{S}\crl{   \vLambda_{i,s} \vJ_s(\vx_i) \vmu_*  - \vr_{i,s} } } },
   \label{eq:tq_*}
\ee
which can be expressed as a product of Gaussian distributions, provided that $\vLambda_{i,s}\succ 0 $. Here we define $N \times S$ observations as $\tvy_{i,s} := \vJ_s(\vx_i)\vmu_* - \vLambda_{i,s}^{-1}\vr_{i,s}$ and get
\be
    \Tilde{q}_*(\vparam) \propto \gauss(\vparam|0, \delta^{-1}\vI_P) \prod_{i=1}^N \prod_{s=1}^S \gauss(\tvy_{i,s} | \vJ_s(\vx_i)\vparam, S \vLambda_{i,s}^{-1}).
\ee
As discussed in the proof of Theorem \ref{thm:laplace_ggn}, the right hand side of the above equation is proportional to the posterior distribution of a linear basis-function model $ \tvy_{i,s} = \vJ_s(\vx_i)\vparam + \vepsilon_{i,s}$ with Gaussian noise $\vepsilon_{i,s} \sim \gauss(0, S \vLambda_{i,s}^{-1})$ and prior distribution $\vparam \sim \gauss(0,\delta^{-1} \vI_P)$. The predictive distribution of this model can be equivalently written in the function space, giving rise to a GP regression model with kernel $\delta^{-1} \vJ_s(\vx) \vJ_{s'}(\vx')^\top$.
\end{proof}
